# Supplementary material for: Competition between phase ordering and phase segregation in the Ti$_x$NbMoTaW and Ti$_x$VNbMoTaW refractory high-entropy alloys
Source: arXiv:2401.16243 ancillary file (2024-03-14)
Supplement: Supplementary file 1 [file supplemental.pdf]

# Competition between phase ordering and phase segregation in the $Ti_x$NbMoTaW and $Ti_x$VNbMoTaW refractory high-entropy alloys

## Supplemental Material

Christopher D. Woodgate* and Julie B. Staunton†
*Department of Physics, University of Warwick, Coventry, CV4 7AL, United Kingdom*
(Dated: March 14, 2024)

This is the supplemental material accompanying the main text. Specifically, we include plots of the difference in total DFT energy between bcc and hcp structures for the disordered solid solutions considered in this work, tables of our fitted atom-atom pairwise interaction parameters, and also plots of the Warren-Cowley ASRO parameters for our Monte Carlo simulations at *second*-nearest-neighbour distance. (The main text only includes results for first-nearest-neighbour distance.)

### I. COMPARISON BETWEEN BCC AND HCP ENERGY

Figures 1 and 2 show the difference in total energy-per-atom between bcc and hcp phases within the KKR-CPA formulation of DFT [1, 2] as implemented in the Hutsepot code [3]. For both systems, across the range of $x$ values considered in this work, the bcc structure is energetically favoured.

### II. FITTED ATOM-ATOM INTERACTION ENERGIES

Tables I - VI provide the fitted atom-atom interactions for the Bragg-Williams Hamiltonian,

$$H(\{\xi_{i\alpha}\}) = \frac{1}{2}\sum_{i,j}\sum_{\alpha\alpha'} V_{i\alpha;j\alpha'}\,\xi_{i\alpha}\xi_{j\alpha'}. \tag{1}$$

from our reciprocal-space data based on a perturbative analysis of the DFT internal energy of the CPA reference medium. Across all compositions, interactions are fitted to the first four coordination shells of the bcc lattice. These interactions are also available in machine-readable format in the open-access dataset associated with this publication, DOI: 10.5281/zenodo.10580621.

### III. WARREN-COWLEY ASRO PARAMETERS ON THE SECOND COORDINATION SHELL

Figures 3 and 4 show plots of the specific heat capacity (SHC) and Warren-Cowley atomic short-range order (ASRO) parameters [4, 5] on the *second* coordination shell as a function of temperature for $Ti_x$NbMoTaW and $Ti_x$VNbMoTaW for a range of values of $x$.

[1] H. Ebert, D. Ködderitzsch, and J. Minár, Reports on Progress in Physics **74**, 096501 (2011).
[2] J. S. Faulkner, G. M. Stocks, and Y. Wang, *Multiple Scattering Theory: Electronic Structure of Solids*, 1st ed. (IOP Publishing, Bristol, UK, 2018).
[3] M. Hoffmann, A. Ernst, W. Hergert, V. N. Antonov, W. A. Adeagbo, R. M. Geilhufe, and H. Ben Hamed, Physica Status Solidi (b) **257**, 1900671 (2020).
[4] J. M. Cowley, Physical Review **77**, 669 (1950).
[5] J. M. Cowley, Physical Review **138**, A1384 (1965).

* Christopher.Woodgate@warwick.ac.uk
† J.B.Staunton@warwick.ac.uk

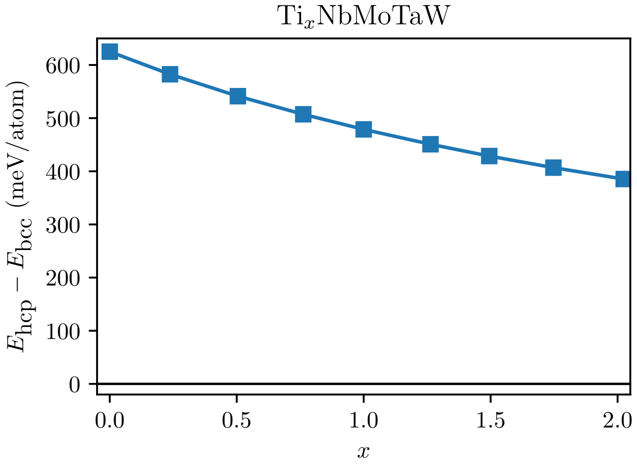


FIG. 1. Comparison of the difference in total energy-per-atom as a function of $x$ for Ti$x$NbMoTaW comparing the bcc and hcp structures, computed using the all-electron KKR-CPA Hutsepot code. Across the range of $x$ considered, bcc is clearly the favoured structure.

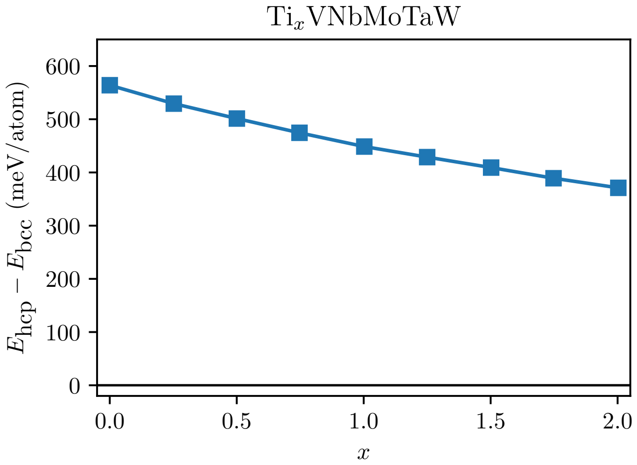


FIG. 2. Comparison of the difference in total energy-per-atom as a function of $x$ for Ti$x$VNbMoTaW comparing the bcc and hcp structures, computed using the all-electron KKR-CPA Hutsepot code. Across the range of $x$ considered, bcc is clearly the favoured structure.

| $V^{(1)}_{\alpha\alpha'}$ | Nb | Mo | Ta | W |
|---|---|---|---|---|
| Nb | 7.4 | −11.9 | 11.7 | −7.2 |
| Mo | −11.9 | 10.5 | −11.5 | 12.9 |
| Ta | 11.7 | −11.5 | 12.2 | −12.4 |
| W | −7.2 | 12.9 | −12.4 | 6.6 |

| $V^{(2)}_{\alpha\alpha'}$ | Nb | Mo | Ta | W |
|---|---|---|---|---|
| Nb | 6.5 | −2.0 | 2.8 | −7.3 |
| Mo | −2.0 | 2.8 | −2.1 | 1.3 |
| Ta | 2.8 | −2.1 | 1.8 | −2.5 |
| W | −7.3 | 1.3 | −2.5 | 8.5 |

| $V^{(3)}_{\alpha\alpha'}$ | Nb | Mo | Ta | W |
|---|---|---|---|---|
| Nb | 0.0 | −1.0 | 0.8 | 0.1 |
| Mo | −1.0 | 2.0 | −2.0 | 0.9 |
| Ta | 0.8 | −2.0 | 1.9 | −0.8 |
| W | 0.1 | 0.9 | −0.8 | −0.2 |

| $V^{(4)}_{\alpha\alpha'}$ | Nb | Mo | Ta | W |
|---|---|---|---|---|
| Nb | −0.0 | −0.3 | 0.2 | 0.2 |
| Mo | −0.3 | 0.2 | −0.2 | 0.3 |
| Ta | 0.2 | −0.2 | 0.1 | −0.1 |
| W | 0.2 | 0.3 | −0.1 | −0.3 |

TABLE I. Fitted pairwise interactions for the NbMoTaW alloy. (*I.e.*, $Ti_x$NbMoTaW, $x = 0$.) The interaction is fitted to the first four coordination shells of the bcc lattice. All energies in units of meV.

| $V^{(1)}_{\alpha\alpha'}$ | Ti | Nb | Mo | Ta | W |
|---|---|---|---|---|---|
| Ti | −48.3 | 12.1 | −25.7 | 32.8 | 5.2 |
| Nb | 12.1 | 4.8 | −9.8 | 7.1 | −8.2 |
| Mo | −25.7 | −9.8 | 17.8 | −11.7 | 16.7 |
| Ta | 32.8 | 7.1 | −11.7 | 4.9 | −16.8 |
| W | 5.2 | −8.2 | 16.7 | −16.8 | 5.6 |

| $V^{(2)}_{\alpha\alpha'}$ | Ti | Nb | Mo | Ta | W |
|---|---|---|---|---|---|
| Ti | 76.5 | 5.2 | −4.5 | −9.6 | −29.7 |
| Nb | 5.2 | 3.0 | −2.9 | 1.8 | −4.5 |
| Mo | −4.5 | −2.9 | 2.5 | −1.4 | 4.1 |
| Ta | −9.6 | 1.8 | −1.4 | 2.9 | 1.5 |
| W | −29.7 | −4.5 | 4.1 | 1.5 | 13.8 |

| $V^{(3)}_{\alpha\alpha'}$ | Ti | Nb | Mo | Ta | W |
|---|---|---|---|---|---|
| Ti | 1.6 | −1.8 | −0.1 | −0.0 | 1.2 |
| Nb | −1.8 | 0.3 | −0.5 | 0.8 | 0.3 |
| Mo | −0.1 | −0.5 | 2.2 | −2.1 | 0.5 |
| Ta | −0.0 | 0.8 | −2.1 | 2.0 | −0.7 |
| W | 1.2 | 0.3 | 0.5 | −0.7 | −0.7 |

| $V^{(4)}_{\alpha\alpha'}$ | Ti | Nb | Mo | Ta | W |
|---|---|---|---|---|---|
| Ti | −11.9 | −0.6 | 2.0 | 0.5 | 4.1 |
| Nb | −0.6 | 0.2 | −0.2 | 0.3 | −0.0 |
| Mo | 2.0 | −0.2 | −0.1 | −0.3 | −0.3 |
| Ta | 0.5 | 0.3 | −0.3 | 0.3 | −0.5 |
| W | 4.1 | −0.0 | −0.3 | −0.5 | −1.2 |

TABLE II. Fitted pairwise interactions for the $Ti_{0.5}$NbMoTaW alloy. (*I.e.*, $Ti_x$NbMoTaW, $x = 0.5$.) The interaction is fitted to the first four coordination shells of the bcc lattice. All energies in units of meV.

| $V^{(1)}_{\alpha\alpha'}$ | Ti | Nb | Mo | Ta | W |
|---|---|---|---|---|---|
| Ti | −46.5 | 16.1 | −18.2 | 36.3 | 12.3 |
| Nb | 16.1 | 1.6 | −9.0 | 1.9 | −10.6 |
| Mo | −18.2 | −9.0 | 22.1 | −13.0 | 18.1 |
| Ta | 36.3 | 1.9 | −13.0 | −3.0 | −22.2 |
| W | 12.3 | −10.6 | 18.1 | −22.2 | 2.5 |

| $V^{(2)}_{\alpha\alpha'}$ | Ti | Nb | Mo | Ta | W |
|---|---|---|---|---|---|
| Ti | 63.0 | −3.4 | −10.3 | −16.3 | −32.9 |
| Nb | −3.4 | 2.3 | −1.6 | 3.0 | −0.3 |
| Mo | −10.3 | −1.6 | 3.5 | 1.1 | 7.3 |
| Ta | −16.3 | 3.0 | 1.1 | 5.6 | 6.7 |
| W | −32.9 | −0.3 | 7.3 | 6.7 | 19.2 |

| $V^{(3)}_{\alpha\alpha'}$ | Ti | Nb | Mo | Ta | W |
|---|---|---|---|---|---|
| Ti | 1.8 | −2.4 | −0.2 | −0.5 | 1.2 |
| Nb | −2.4 | 0.7 | −0.0 | 1.0 | 0.7 |
| Mo | −0.2 | −0.0 | 2.1 | −2.0 | 0.1 |
| Ta | −0.5 | 1.0 | −2.0 | 2.1 | −0.6 |
| W | 1.2 | 0.7 | 0.1 | −0.6 | −1.3 |

| $V^{(4)}_{\alpha\alpha'}$ | Ti | Nb | Mo | Ta | W |
|---|---|---|---|---|---|
| Ti | −8.5 | 0.1 | 2.7 | 1.2 | 4.5 |
| Nb | 0.1 | 0.3 | −0.3 | 0.2 | −0.3 |
| Mo | 2.7 | −0.3 | −0.6 | −0.6 | −1.1 |
| Ta | 1.2 | 0.2 | −0.6 | 0.1 | −0.9 |
| W | 4.5 | −0.3 | −1.1 | −0.9 | −2.2 |

TABLE III. Fitted pairwise interactions for the TiNbMoTaW alloy. (*I.e.*, $Ti_x$NbMoTaW, $x = 1$.) The interaction is fitted to the first four coordination shells of the bcc lattice. All energies in units of meV.

| $V^{(1)}_{\alpha\alpha'}$ | V | Nb | Mo | Ta | W |
|---|---|---|---|---|---|
| V | −28.0 | 5.4 | −14.0 | 24.2 | 12.4 |
| Nb | 5.4 | 5.7 | −8.5 | 6.7 | −9.3 |
| Mo | −14.0 | −8.5 | 19.1 | −12.5 | 16.0 |
| Ta | 24.2 | 6.7 | −12.5 | 2.4 | −20.9 |
| W | 12.4 | −9.3 | 16.0 | −20.9 | 1.7 |

| $V^{(2)}_{\alpha\alpha'}$ | V | Nb | Mo | Ta | W |
|---|---|---|---|---|---|
| V | 50.9 | −2.7 | −4.6 | −16.0 | −27.5 |
| Nb | −2.7 | 4.2 | −3.7 | 4.8 | −2.5 |
| Mo | −4.6 | −3.7 | 3.2 | −1.4 | 6.5 |
| Ta | −16.0 | 4.8 | −1.4 | 7.9 | 4.7 |
| W | −27.5 | −2.5 | 6.5 | 4.7 | 18.8 |

| $V^{(3)}_{\alpha\alpha'}$ | V | Nb | Mo | Ta | W |
|---|---|---|---|---|---|
| V | 1.8 | −1.2 | 0.1 | −0.8 | 0.1 |
| Nb | −1.2 | 0.5 | −0.9 | 1.3 | 0.2 |
| Mo | 0.1 | −0.9 | 2.4 | −2.5 | 0.8 |
| Ta | −0.8 | 1.3 | −2.5 | 2.8 | −0.8 |
| W | 0.1 | 0.2 | 0.8 | −0.8 | −0.3 |

| $V^{(4)}_{\alpha\alpha'}$ | V | Nb | Mo | Ta | W |
|---|---|---|---|---|---|
| V | −7.4 | 0.4 | 1.9 | 1.3 | 3.8 |
| Nb | 0.4 | 0.2 | −0.5 | 0.3 | −0.4 |
| Mo | 1.9 | −0.5 | 0.2 | −1.0 | −0.5 |
| Ta | 1.3 | 0.3 | −1.0 | 0.4 | −1.1 |
| W | 3.8 | −0.4 | −0.5 | −1.1 | −1.8 |

TABLE IV. Fitted pairwise interactions for the VNbMoTaW alloy. (*I.e.*, $Ti_x$VNbMoTaW, $x = 0$.) The interaction is fitted to the first four coordination shells of the bcc lattice. All energies in units of meV.

| $V^{(1)}_{\alpha\alpha'}$ | Ti | V | Nb | Mo | Ta | W |
|---|---|---|---|---|---|---|
| Ti | −30.1 | −35.8 | 20.8 | −19.8 | 40.9 | 8.9 |
| V | −35.8 | −29.6 | 7.7 | −5.8 | 25.5 | 19.8 |
| Nb | 20.8 | 7.7 | 1.9 | −8.6 | 1.0 | −12.3 |
| Mo | −19.8 | −5.8 | −8.6 | 22.4 | −14.6 | 16.4 |
| Ta | 40.9 | 25.5 | 1.0 | −14.6 | −5.7 | −26.5 |
| W | 8.9 | 19.8 | −12.3 | 16.4 | −26.5 | −1.8 |

| $V^{(2)}_{\alpha\alpha'}$ | Ti | V | Nb | Mo | Ta | W |
|---|---|---|---|---|---|---|
| Ti | 61.7 | 45.9 | −5.7 | −15.3 | −18.1 | −37.4 |
| V | 45.9 | 41.6 | −8.3 | −8.1 | −19.6 | −28.3 |
| Nb | −5.7 | −8.3 | 4.2 | −1.5 | 6.2 | 2.1 |
| Mo | −15.3 | −8.1 | −1.5 | 4.9 | 1.9 | 10.3 |
| Ta | −18.1 | −19.6 | 6.2 | 1.9 | 10.4 | 10.0 |
| W | −37.4 | −28.3 | 2.1 | 10.3 | 10.0 | 24.4 |

| $V^{(3)}_{\alpha\alpha'}$ | Ti | V | Nb | Mo | Ta | W |
|---|---|---|---|---|---|---|
| Ti | 1.8 | 2.8 | −2.5 | −1.1 | −0.4 | 0.4 |
| V | 2.8 | 3.4 | −2.0 | −0.0 | −2.0 | −0.7 |
| Nb | −2.5 | −2.0 | 1.1 | −0.2 | 1.6 | 0.8 |
| Mo | −1.1 | −0.0 | −0.2 | 2.4 | −2.2 | 0.6 |
| Ta | −0.4 | −2.0 | 1.6 | −2.2 | 3.1 | −0.4 |
| W | 0.4 | −0.7 | 0.8 | 0.6 | −0.4 | −0.5 |

| $V^{(4)}_{\alpha\alpha'}$ | Ti | V | Nb | Mo | Ta | W |
|---|---|---|---|---|---|---|
| Ti | −9.1 | −6.5 | 0.7 | 3.1 | 2.0 | 5.2 |
| V | −6.5 | −5.0 | 0.8 | 2.1 | 1.7 | 3.6 |
| Nb | 0.7 | 0.8 | 0.1 | −0.6 | 0.0 | −0.7 |
| Mo | 3.1 | 2.1 | −0.6 | −0.4 | −1.3 | −1.3 |
| Ta | 2.0 | 1.7 | 0.0 | −1.3 | 0.0 | −1.5 |
| W | 5.2 | 3.6 | −0.7 | −1.3 | −1.5 | −2.7 |

TABLE V. Fitted pairwise interactions for the $Ti_{0.5}$VNbMoTaW alloy. (*I.e.*, $Ti_x$VNbMoTaW, $x = 0.5$.) The interaction is fitted to the first four coordination shells of the bcc lattice. All energies in units of meV.

| $V^{(1)}_{\alpha\alpha'}$ | Ti | V | Nb | Mo | Ta | W |
|---|---|---|---|---|---|---|
| Ti | −29.5 | −36.6 | 23.3 | −13.5 | 42.5 | 14.4 |
| V | −36.6 | −29.3 | 10.5 | 1.8 | 27.6 | 26.9 |
| Nb | 23.3 | 10.5 | −2.6 | −9.7 | −5.6 | −16.5 |
| Mo | −13.5 | 1.8 | −9.7 | 24.0 | −17.5 | 15.1 |
| Ta | 42.5 | 27.6 | −5.6 | −17.5 | −14.8 | −33.2 |
| W | 14.4 | 26.9 | −16.5 | 15.1 | −33.2 | −7.0 |

| $V^{(2)}_{\alpha\alpha'}$ | Ti | V | Nb | Mo | Ta | W |
|---|---|---|---|---|---|---|
| Ti | 51.3 | 37.4 | −11.3 | −18.2 | −22.4 | −38.1 |
| V | 37.4 | 34.6 | −12.3 | −9.9 | −22.5 | −28.2 |
| Nb | −11.3 | −12.3 | 5.8 | 1.6 | 9.1 | 7.4 |
| Mo | −18.2 | −9.9 | 1.6 | 6.7 | 6.0 | 14.1 |
| Ta | −22.4 | −22.5 | 9.1 | 6.0 | 14.3 | 16.0 |
| W | −38.1 | −28.2 | 7.4 | 14.1 | 16.0 | 29.8 |

| $V^{(3)}_{\alpha\alpha'}$ | Ti | V | Nb | Mo | Ta | W |
|---|---|---|---|---|---|---|
| Ti | 1.3 | 2.7 | −3.0 | −1.0 | −0.8 | 0.6 |
| V | 2.7 | 3.6 | −2.6 | −0.1 | −2.8 | −1.0 |
| Nb | −3.0 | −2.6 | 1.7 | 0.5 | 2.0 | 1.4 |
| Mo | −1.0 | −0.1 | 0.5 | 2.3 | −1.8 | 0.1 |
| Ta | −0.8 | −2.8 | 2.0 | −1.8 | 3.4 | −0.0 |
| W | 0.6 | −1.0 | 1.4 | 0.1 | −0.0 | −1.1 |

| $V^{(4)}_{\alpha\alpha'}$ | Ti | V | Nb | Mo | Ta | W |
|---|---|---|---|---|---|---|
| Ti | −6.8 | −4.7 | 1.0 | 3.3 | 2.2 | 5.2 |
| V | −4.7 | −3.7 | 1.1 | 2.2 | 1.8 | 3.5 |
| Nb | 1.0 | 1.1 | −0.0 | −0.7 | −0.3 | −1.1 |
| Mo | 3.3 | 2.2 | −0.7 | −1.1 | −1.5 | −2.2 |
| Ta | 2.2 | 1.8 | −0.3 | −1.5 | −0.3 | −1.9 |
| W | 5.2 | 3.5 | −1.1 | −2.2 | −1.9 | −3.7 |

TABLE VI. Fitted pairwise interactions for the TiVNbMoTaW alloy. (*I.e.*, $Ti_x$VNbMoTaW, $x = 1$.) The interaction is fitted to the first four coordination shells of the bcc lattice. All energies in units of meV.

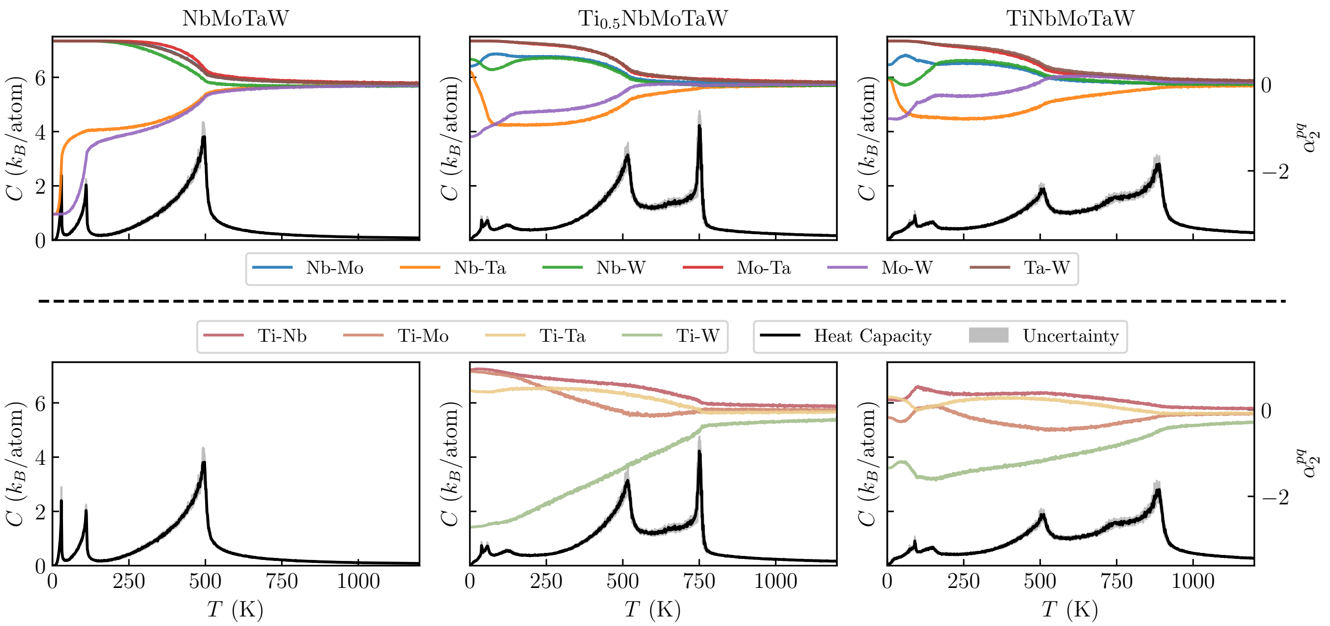


FIG. 3. Plots of the SHC and Warren-Cowley ASRO parameters on the second coordination shell for Ti$_x$NbMoTaW.

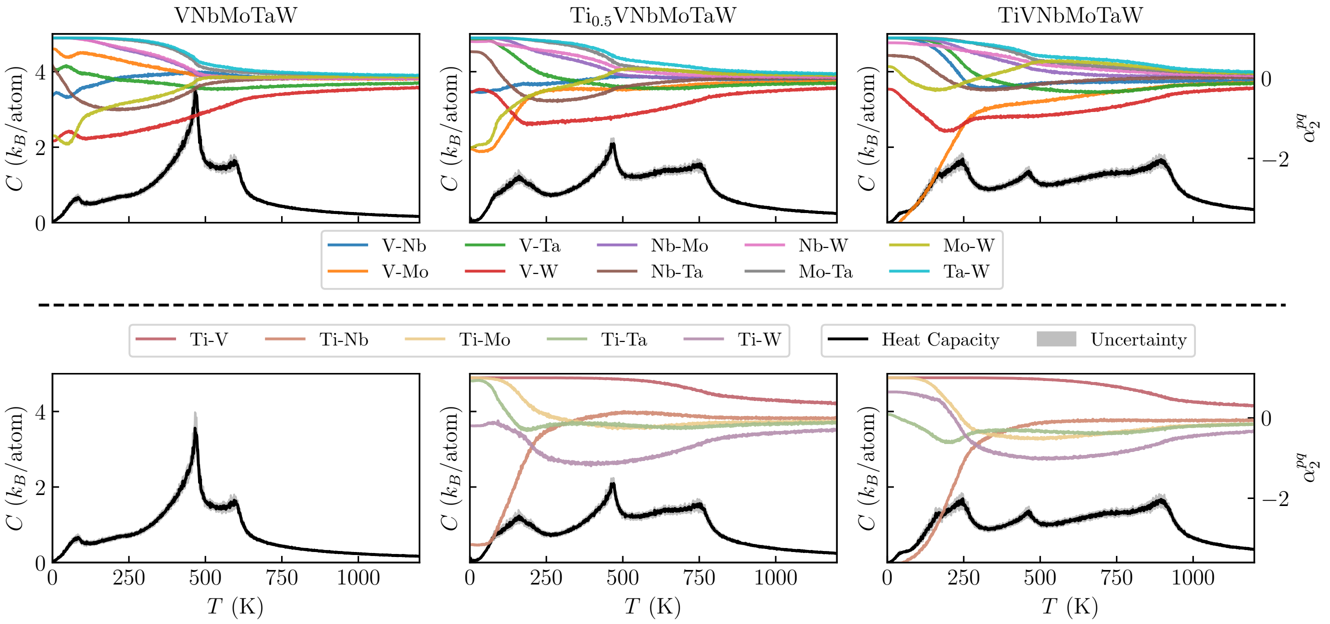


FIG. 4. Plots of the SHC and Warren-Cowley ASRO parameters on the second coordination shell for Ti$_x$VNbMoTaW.
